# Supplementary material for: PC-JeDi: Diffusion for Particle Cloud Generation in High Energy Physics
Source: arXiv:2303.05376 source file (2024-02-21)
Supplement: Supplementary file 1 [file appendix_results_condition.tex]

\begin{figure}[hbpt]
    \centering
    \begin{subfigure}{.5\textwidth}
        \centering
        \includegraphics[width=1.\linewidth]{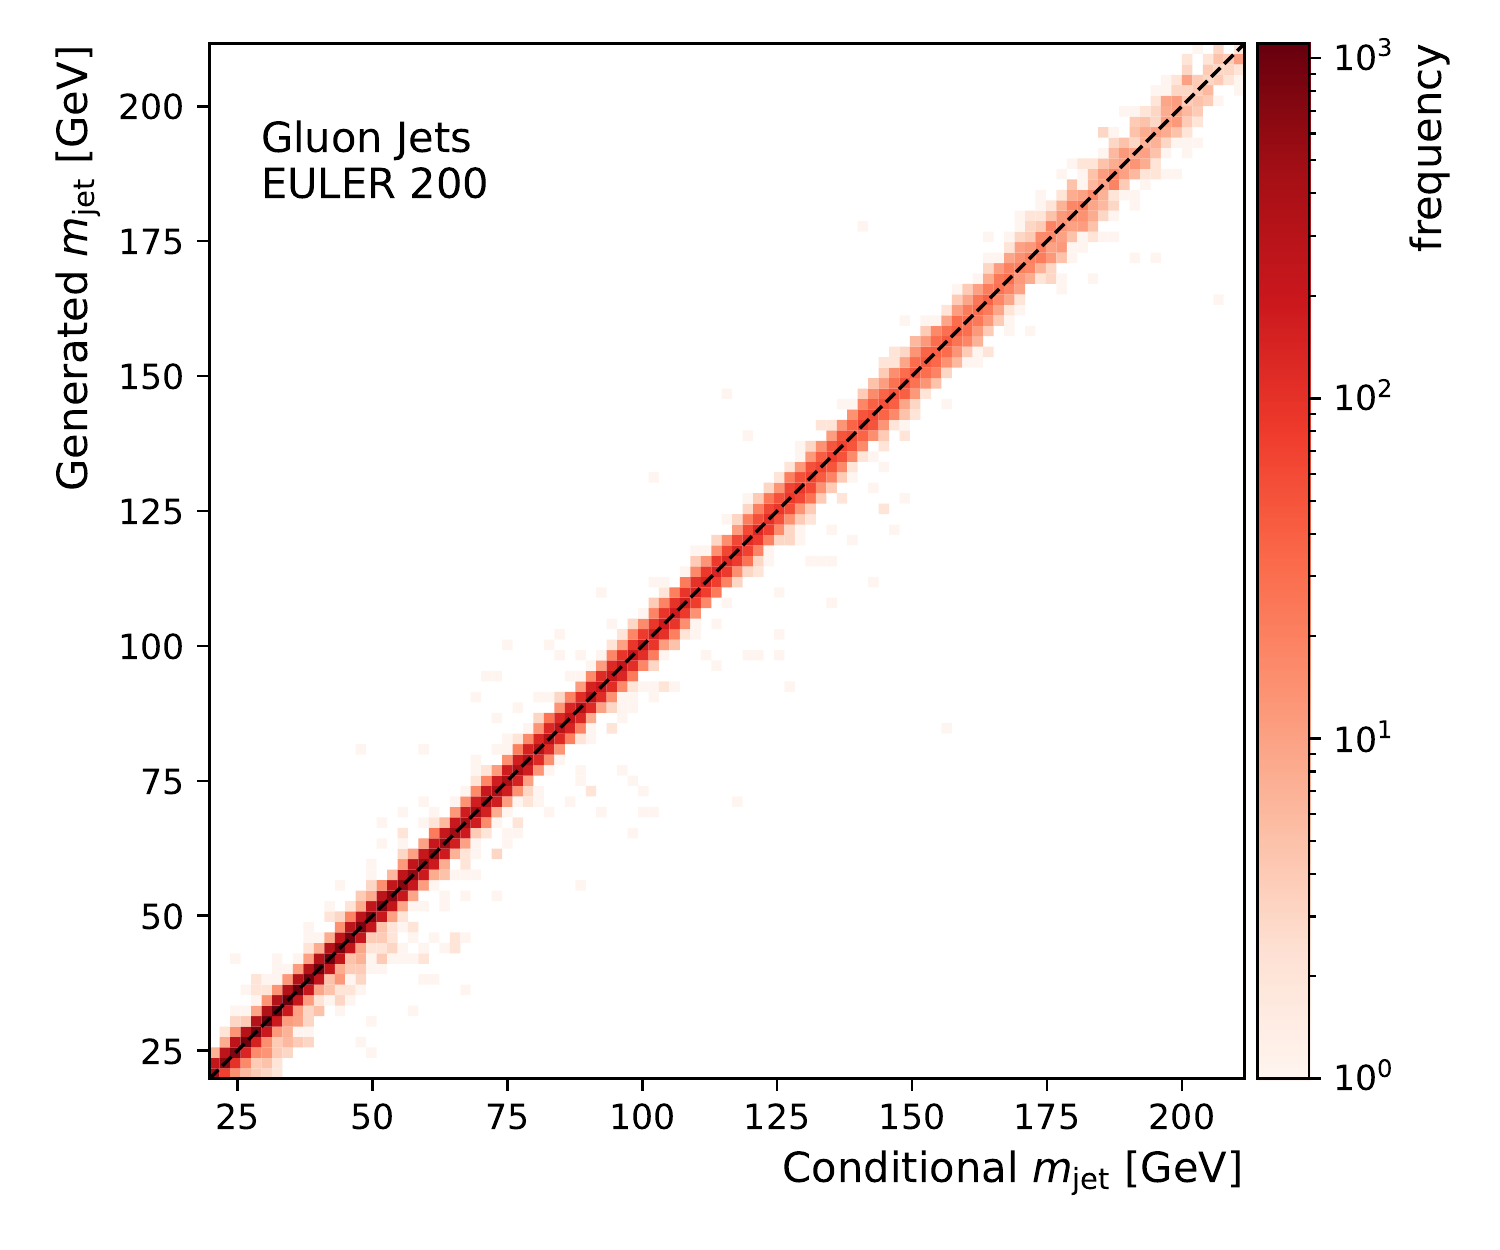}
    \end{subfigure}%
    \begin{subfigure}{.5\textwidth}
        \centering
        \includegraphics[width=1.\linewidth]{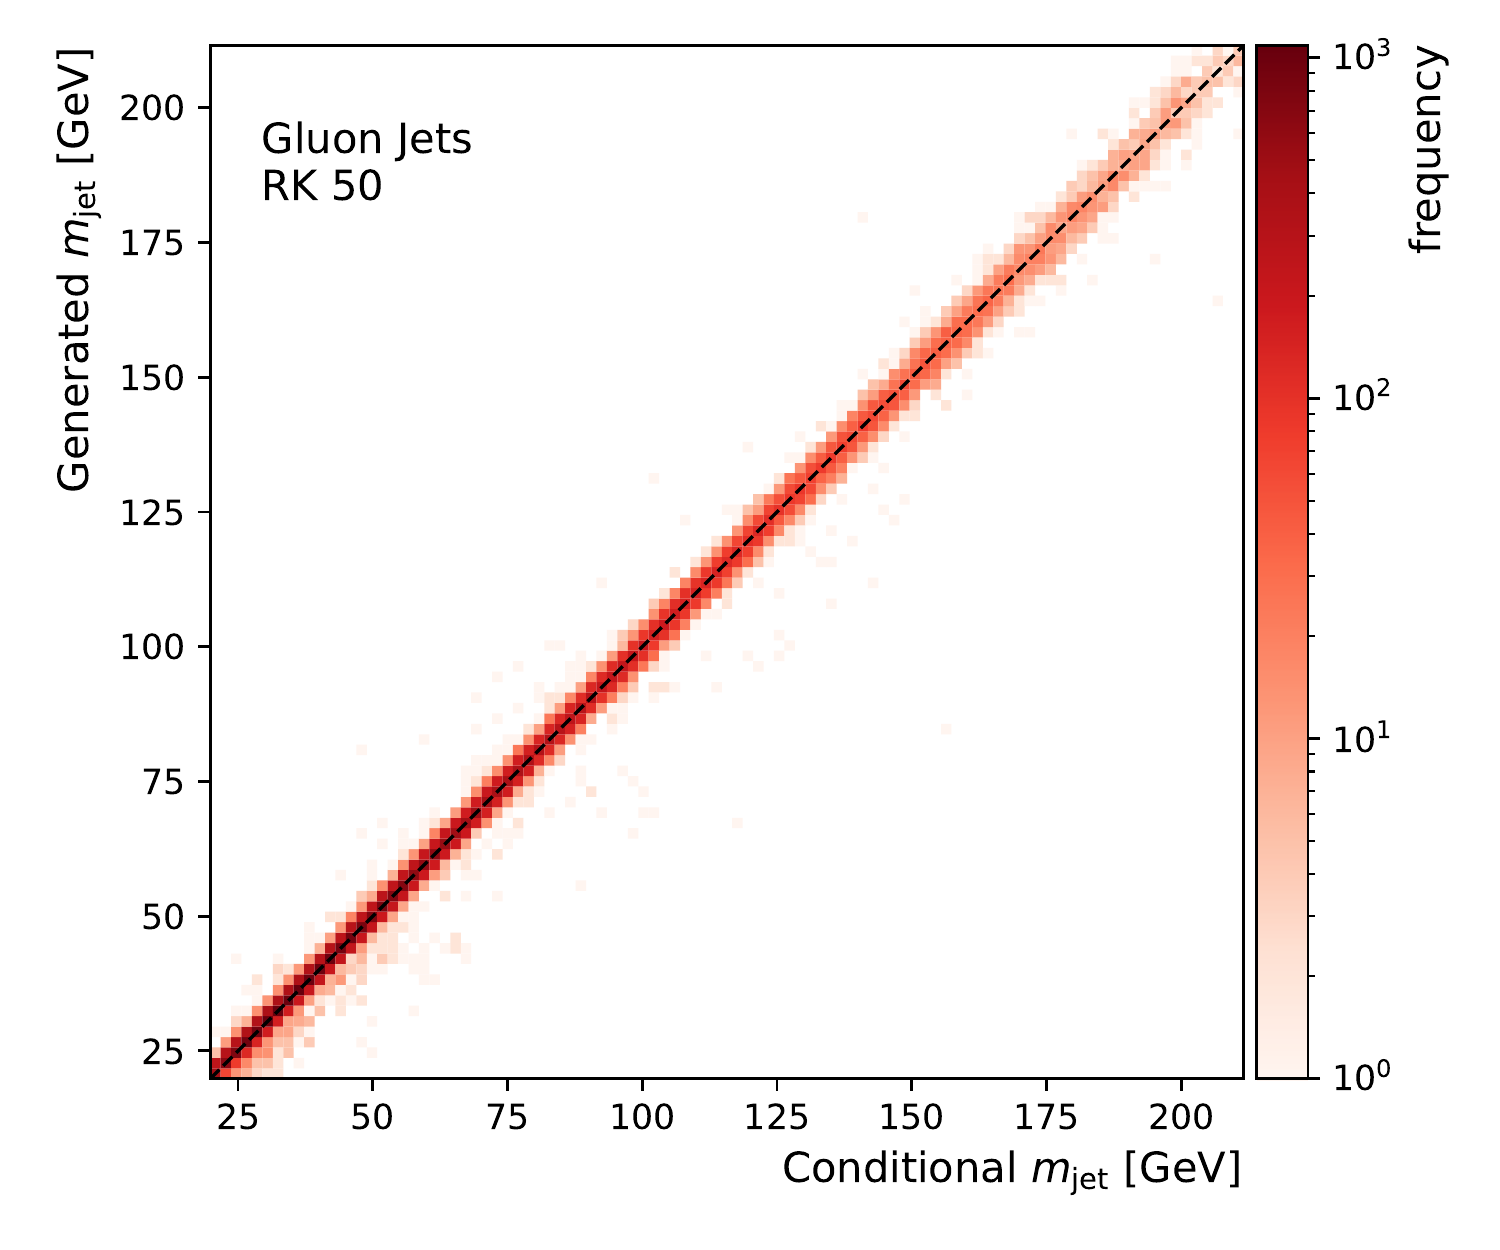}
    \end{subfigure}% \\
    \caption{Two-dimensional histograms showing the correlation between the conditional and generated jet mass for the gluon jets using Euler and RK solvers.}
    \label{fig:gluon_mass_heatmap_app}
\end{figure}

\begin{figure}[hbpt]
    \centering
    \begin{subfigure}{.5\textwidth}
        \centering
        \includegraphics[width=1.\linewidth]{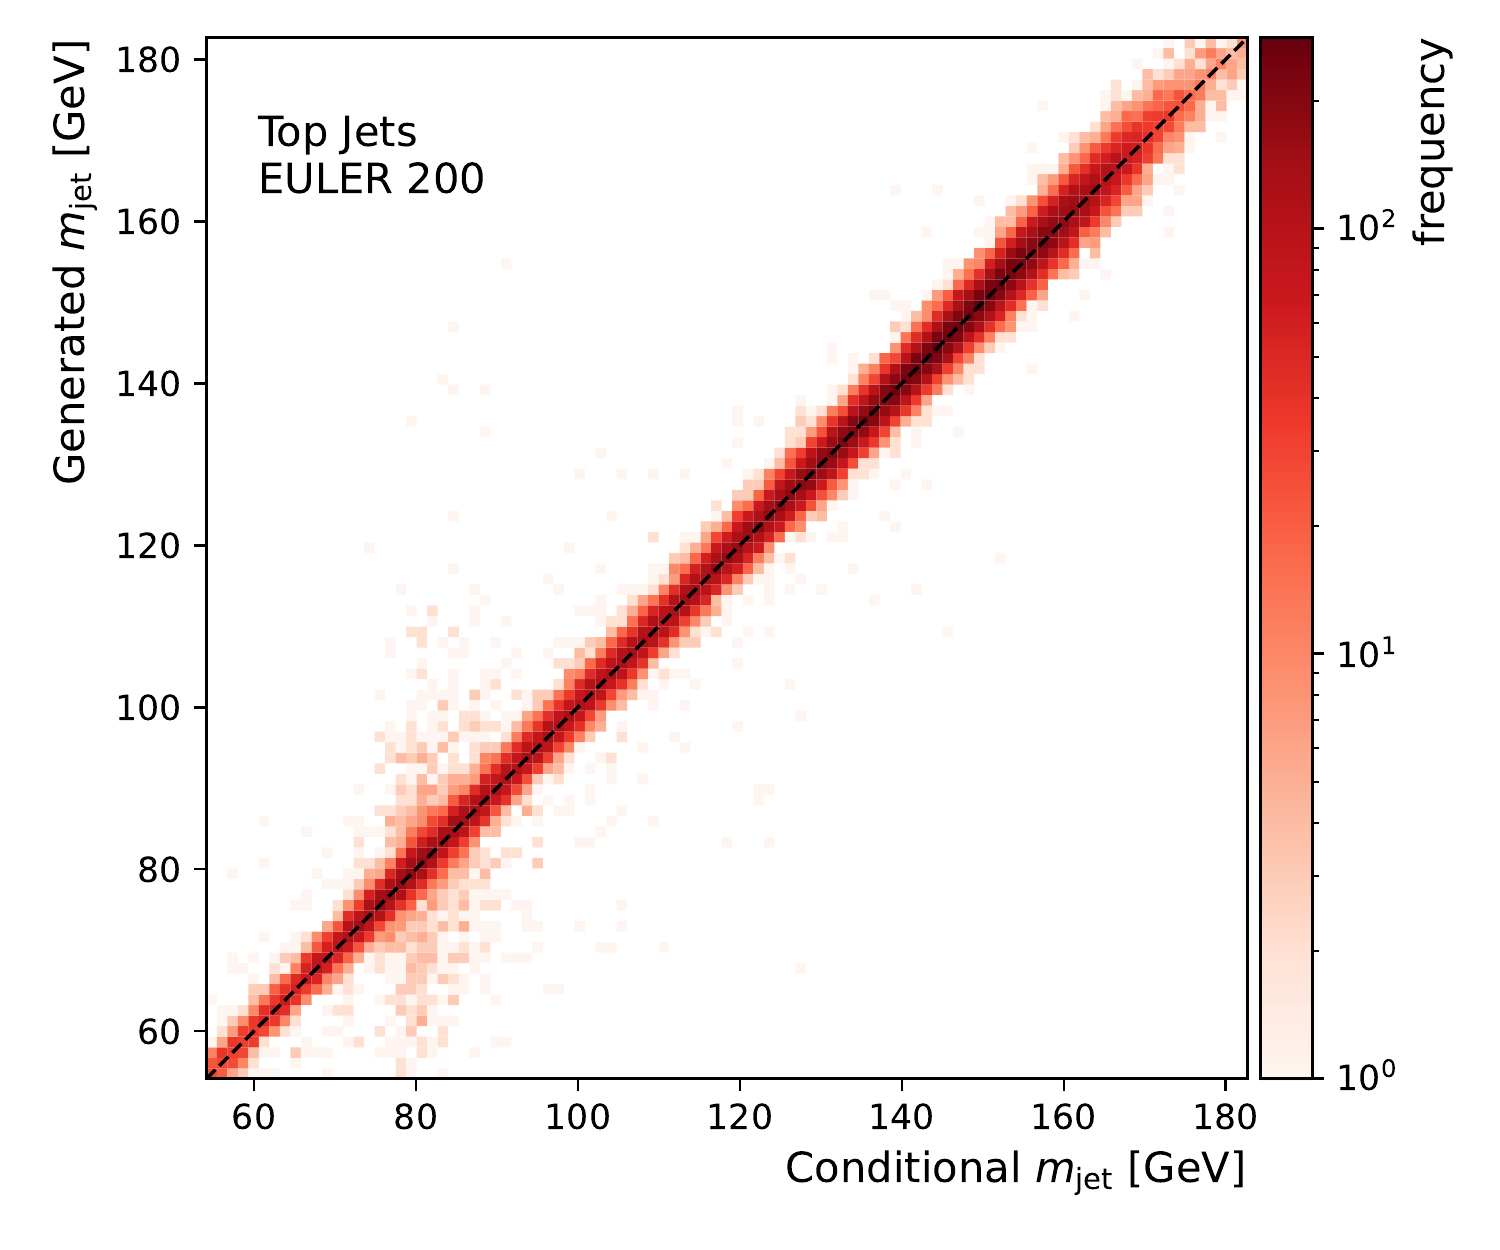}
    \end{subfigure}%
    \begin{subfigure}{.5\textwidth}
        \centering
        \includegraphics[width=1.\linewidth]{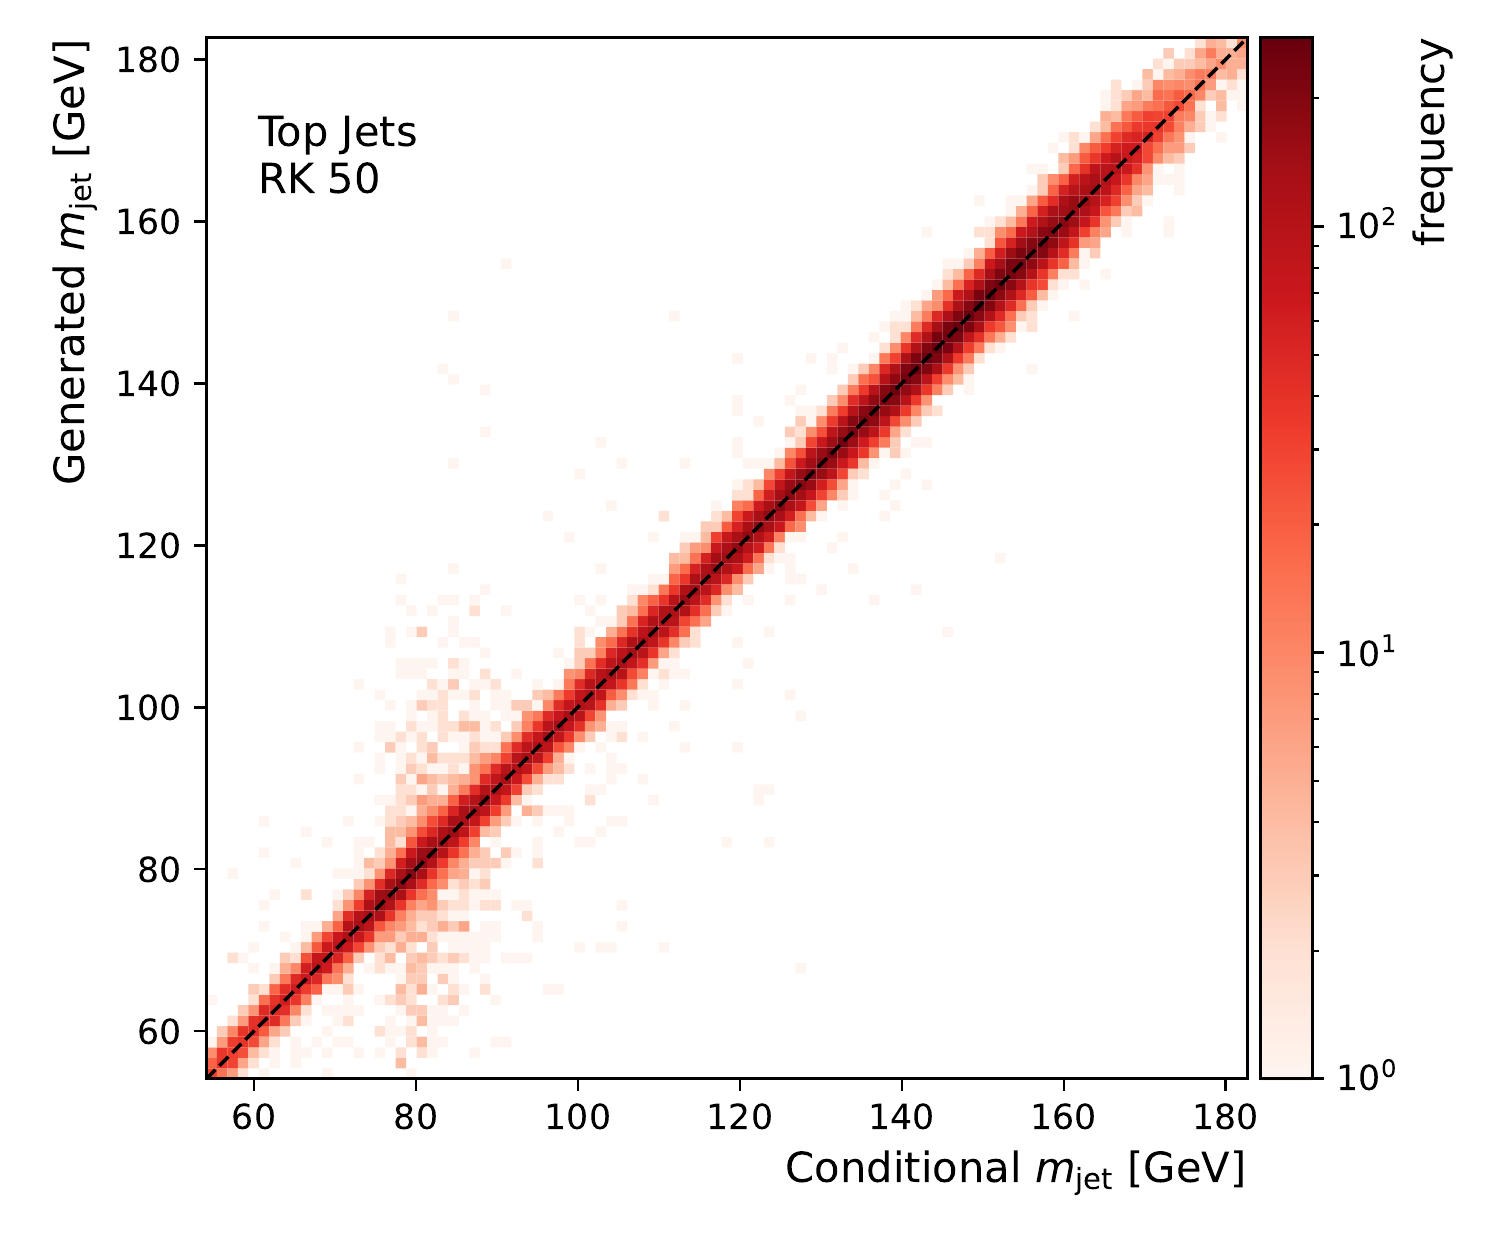}
    \end{subfigure}% \\
    \caption{Two-dimensional histograms showing the correlation between the conditional and generated jet mass for the top jets using Euler and RK solvers.}
    \label{fig:top_mass_heatmap_app}
\end{figure}

\begin{figure}[hbpt]
    \centering
    \begin{subfigure}{.5\textwidth}
        \centering
        \includegraphics[width=1.\linewidth]{figures/gluon_generation/jet_pt_corr_heatmap_euler_200_abs.pdf}
    \end{subfigure}%
    \begin{subfigure}{.5\textwidth}
        \centering
        \includegraphics[width=1.\linewidth]{figures/gluon_generation/jet_pt_corr_heatmap_rk_50_abs.pdf}
    \end{subfigure}% \\
    \caption{Two-dimensional histograms showing the correlation between the conditional and generated jet transverse momenta for the gluon jets using Euler and RK solvers.}
    \label{fig:gluon_pt_heatmap_app}
\end{figure}

\begin{figure}[hbpt]
    \centering
    \begin{subfigure}{.5\textwidth}
        \centering
        \includegraphics[width=1.\linewidth]{figures/top_generation/jet_pt_corr_heatmap_euler_200_abs.pdf}
    \end{subfigure}%
    \begin{subfigure}{.5\textwidth}
        \centering
        \includegraphics[width=1.\linewidth]{figures/top_generation/jet_pt_corr_heatmap_rk_50_abs.pdf}
    \end{subfigure}% \\
    \caption{Two-dimensional histograms showing the correlation between the conditional and generated jet transverse momenta for the top jets using Euler and RK solvers.}
    \label{fig:top_pt_heatmap_app}
\end{figure}
